# Supplementary material for: Topological Solitons in Square-root Graphene Nanoribbons Controlled by Electric Fields
Source: arXiv:2406.13978 ancillary file (2024-06-20)
Supplement: Supplementary file 1 [file Supplementary.pdf]

# Supplementary Materials for Topological Solitons in Square-root Graphene Nanoribbons Controlled by Electric Fields

Haiyue Huang<sup>1†</sup>, Mamun Sarker<sup>2†</sup>, Percy Zahl<sup>3</sup>,  
C. Stephen Hellberg<sup>4</sup>, Jeremy Levy<sup>5</sup>, Ioannis Petrides<sup>1\*</sup>,  
Alexander Sinitskii<sup>2\*</sup>, Prineha Narang<sup>1,6\*</sup>

<sup>1</sup>Division of Physical Sciences, College of Letters and Science, University  
of California, Los Angeles, 90095, California, USA.

<sup>2</sup>Department of Chemistry, University of Nebraska, Lincoln, 68588,  
Nebraska, USA.

<sup>3</sup>Center for Functional Nanomaterials, Brookhaven National Laboratory,  
Upton, 11973, New York, USA.

<sup>4</sup>U.S. Naval Research Laboratory, Washington, 20375, District of  
Columbia, USA.

<sup>5</sup>Department of Physics and Astronomy, University of Pittsburgh,  
Pittsburgh, 15260, Pennsylvania, USA.

<sup>6</sup>Department of Electrical and Computer Engineering, University of  
California, Los Angeles, 90095, California, USA.

\*Corresponding author(s). E-mail(s): [ipetrides@g.ucla.edu](mailto:ipetrides@g.ucla.edu);  
[sinitskii@unl.edu](mailto:sinitskii@unl.edu); [prineha@ucla.edu](mailto:prineha@ucla.edu);

Contributing authors: [haiyuehuang@g.ucla.edu](mailto:haiyuehuang@g.ucla.edu); [msarker2@unl.edu](mailto:msarker2@unl.edu);  
[pzahl@bnl.gov](mailto:pzahl@bnl.gov); [carl.s.hellberg.civ@us.navy.mil](mailto:carl.s.hellberg.civ@us.navy.mil); [jlevy@pitt.edu](mailto:jlevy@pitt.edu);

<sup>†</sup>These authors contributed equally to this work.

## 1 Synthesis of molecular precursor

General: All the starting materials and reagents used were purchased from commercial  
sources and used without further purification unless otherwise noted. The dry solvent  
1,2-dichloro-ethane (DCE) was freshly distilled, employing a standard method before

use. Chemical shifts are stated in parts per million (ppm,  $\delta$ ), downfield from tetramethyl silane (TMS,  $\delta = 0.00$  ppm) and are referenced to residual solvent ( $\text{CDCl}_3$ ,  $\delta = 7.26$  ppm ( $^1\text{H}$ ) and 77.00 ppm ( $^{13}\text{C}$ )). Mass spectrum was collected using Bruker Solari X.

Monomer-T was synthesized following the method previously described by Jacobse, Sarker, and Saxena et al[1]. As shown in Scheme S1, in the first step, 1 (1080.5 mg, 2.0 mmol), and 2-amino-3,6-dimethylbenzoic acid (346.9 mg, 2.1 mmol) were added to a two-neck round bottom flask with a magnetic stirring bar, followed by 10 mL of 1,2-dichloro-ethane (DCE). The mixture was heated to 90°C with constant stirring. A solution of isopentyl nitrite (0.6 mL, 4.6 mmol) in 4 mL DCE was slowly added into the reaction mixture via syringe, and stirring was continued for approximately 30 minutes leading to a color change. After cooling to room temperature, the solvent evaporated, and the residue was precipitated out using hexanes. The precipitate was filtered and washed with hexanes and dried under vacuum, yielding a light-yellow powder. In the second step, the crude powder was transferred to a reaction tube, followed by the addition of 1.0 mL of diphenyl ether and heated to reflux for 30 minutes. The reaction mixture turned dark brown in color and was cooled to room temperature. Purification by flash column chromatography using 10% of dichloromethane (DCM) in hexanes as eluent ( $R_f = 0.61$ ) to give monomer-T as a pale-yellow powder (678 mg, 55% yield).

$^1\text{H}$ -NMR (400 MHz,  $\text{CDCl}_3$ ,  $\delta$ ): 7.99 (d, 2H, and Ar-H), 7.52-7.42 (m, 10H, and Ar-H), 7.39 (d, 1H, and Ar-H), 7.36 (d, 1H, and Ar-H), 7.14 (s, 2H, and Ar-H), 7.11 (d, 2H, and Ar-H), and 1.82 (s, 6H, and methyl-H) ppm.

$^{13}\text{C}$ -NMR (100 MHz,  $\text{CDCl}_3$ , and  $\delta$ ): 142.29, 135.21, 134.50, 133.54, 133.21, 132.96, 132.81, 130.15, 129.73, 129.47, 129.10, 128.23, 125.89, 124.70, 120.08, and 23.65 (methyl-C), ppm.

HR-MS (MALDI FT-ICR, TCNQ Matrix),  $m/z$ : 614.02208 (calculated  $m/z = 614.02448$ ). MALDI FT-ICR and NMR spectra are provided in Fig. S1-S3.

## 2 Square-root tight-binding model

Here we consider the square-root tight-binding model given in Eq.1, the energy levels of the four bands are:

$$E(k) = \pm \sqrt{m^2 + (t_1)^2 + (t_2)^2 \pm 2t_1 \sqrt{m^2 + (t_2)^2} \cos^2 \frac{k}{2}} \quad (1)$$

The model has a chiral symmetry  $\Gamma H \Gamma^\dagger = -H$  characterized by the operator

$$\Gamma = \begin{pmatrix} 0 & 0 & 1 & 0 \\ 0 & 0 & 0 & -1 \\ 1 & 0 & 0 & 0 \\ 0 & -1 & 0 & 0 \end{pmatrix} \quad (2)$$

the matrix of the operator is written in the canonical convention [2], and is  $k$  dependent if written in the periodic convention. The chiral symmetry is thus nonsymmorphic in

61 nature [3]. The time-reversal symmetry is satisfied by  $TH(k)T = H^*(k)$ , with

$$T = \begin{pmatrix} 0 & 0 & 0 & 1 \\ 0 & 0 & 1 & 0 \\ 0 & 1 & 0 & 0 \\ 1 & 0 & 0 & 0 \end{pmatrix} \quad (3)$$

62 Therefore, the system can be categorized to the BDI class according to [4]. It also has  
63 a spatial mirror symmetry  $MH(k)M = H(-k)$ , with

$$M = \begin{pmatrix} 0 & 0 & 0 & 1 \\ 0 & 0 & 1 & 0 \\ 0 & 1 & 0 & 0 \\ 1 & 0 & 0 & 0 \end{pmatrix} \quad (4)$$

64 The Zak phase is a value dependent on the choice of unit cell and the location of  
65 origin. In this work the unit cell is the one drawn in Fig. 1d and the origin is set to  
66 the center of the unit cell. Under this circumstance, the mirror symmetry requires Zak  
67 phase for each band:

$$\gamma_1, \gamma_2, \gamma_3, \gamma_4 \in \{0, \pi\} \text{ mod } 2\pi \quad (5)$$

68 And the chiral symmetry requires:

$$\gamma_4 - \gamma_1 = \gamma_3 - \gamma_2 = \pi \text{ mod } 2\pi \quad (6)$$

69 There are in total four possible combinations of Zak phase, according to Eq. 5 and 6  
70 (Table 1).

71 In the four-lattice square-root model, all of the four possibilities can be achieved  
72 by controlling the sign of  $m$  and  $(m^2 + t_2^2 - t_1^2)$  [5], as elaborated in Table 2. From  
73 the table, we see that when keeping  $t_1$  and  $t_2$  constant, switching the sign of  $m$  always  
74 alternates the Zak phase. This means that  $(\gamma_1 + \gamma_2 + \gamma_3)$  also alternates, whereas  
75  $\gamma_1 + \gamma_2$  remains constant. Therefore, it is the finite gaps, instead of the central gap,  
76 that can host topologically protected boundary state. Meanwhile, the SSH model can  
77 be regarded as a special case of the square-root model where  $m$  equals zero. The  
78 observation that the topological phase at half-filling depends on  $|t_2| - |t_1|$  is consistent  
79 with the previous report [6].

**Table 1** Possible combinations of Zak phase from symmetry considerations

| Case | $\gamma_1$ | $\gamma_2$ | $\gamma_3$ | $\gamma_4$ |
|------|------------|------------|------------|------------|
| A    | 0          | $\pi$      | 0          | $\pi$      |
| B    | $\pi$      | 0          | $\pi$      | 0          |
| C    | $\pi$      | $\pi$      | 0          | 0          |
| D    | 0          | 0          | $\pi$      | $\pi$      |

**Table 2** Zak phase in the square-root model

| Case | Sgn( $m$ ) | Sgn( $m^2 + t_2^2 - t_1^2$ ) |
|------|------------|------------------------------|
| A    | +          | −                            |
| B    | −          | −                            |
| C    | −          | +                            |
| D    | +          | +                            |

**Table 3** Zak phase for the middle four bands in GNR

| pzc-GNR             |                |                |                |                |
|---------------------|----------------|----------------|----------------|----------------|
| Sgn(Electric field) | $\gamma_{153}$ | $\gamma_{154}$ | $\gamma_{155}$ | $\gamma_{156}$ |
| +                   | $\pi$          | $\pi$          | 0              | 0              |
| −                   | 0              | 0              | $\pi$          | $\pi$          |
| 7-AGNR-S(1,3)       |                |                |                |                |
| Sgn(Electric field) | $\gamma_{203}$ | $\gamma_{204}$ | $\gamma_{205}$ | $\gamma_{206}$ |
| +                   | 0              | $\pi$          | 0              | $\pi$          |
| −                   | $\pi$          | 0              | $\pi$          | 0              |

### 3 Constructing effective square-root model in pzc-GNR

The Zak phase in the main text is calculated in two ways. One is utilizing Eq.4 by comparing the parity of the wave function, which gives the Zak phase for the middle four bands (Table 3). Another one is the Wannier charge center method based on DFT results, which can yield a result encompassing contributions from all low-lying bands. We note here that the two results are consistent. To get meaningful parameters ( $m, t_1, t_2$ ) to describe GNR, we first notice that the pattern in Table 3 matches that of case C and D in Table 1. As C and D can be achieved by letting  $|t_1| < |t_2|$  (see Table 2), we next compare the results of square-root model to that of pzc-GNR, assuming  $0 > t_1 > t_2$ . The parameters  $t_1, t_2, m$  in Eq.1 are chosen such that its gap width at the edge and middle of the Brillouin zone is the same as the band structure of GNR calculated by DFT methods. Meanwhile, we assume a positive  $m$  for GNRs under a positive field along the direction shown in Fig. 1. The results are shown in Fig. S4, which demonstrates good agreement between the two band structures. In addition, the hopping parameters for the GNR with and without electric field are very close, further suggesting it is reasonable to use a square-root Hamiltonian to predict properties of GNRs.

In Fig 2, the parity of wave functions is obtained by solving the tight-binding model carried out with the PythTB package [7] assuming only nearest-neighbor hopping

between carbon atoms. The hopping parameter is set to -2.7 eV. To simulate the effects of electric field, we assume an on-site potential proportional to the distance of the atom to the center along the  $y$  axis, i.e.,  $E \cdot (y - y_c)$ , where  $E$  is the strength of the field set to 0 for Fig. S5a,  $+0.05\text{V}/\text{\AA}$  for Fig. S5c, and  $-0.05\text{V}/\text{\AA}$  for Fig. S5j,  $y$  is the vertical coordinate of the carbon and  $y_c$  is the vertical coordinate of the center carbon atom. Fig. S5d, S5k are replicates of Fig. 2b and 2f. For comparison, in Fig. S5h plotted the band structure from the DFT calculations again. The band structures of pzc-GNR in Fig. S5a and Fig. S5h are quite similar. The tight-binding results show gap opening at the middle of the Brillouin zone, especially for the four bands near the Fermi level.

At  $k = \pi/b$ , the parity for all four bands in GNRs are the same as in the square-root model at both negative and positive fields (see Fig. S5d and S5g, S5k and S5n). Now what's different between the two is the parity at  $k = 0$  (see Fig. S5b and S5e, S5i and S5l), which results in different Zak phase. This is due to the fact that at gamma point, the transverse electric field does not affect much of the band structure. The parity of wave functions at  $k = 0$  is mainly determined by the specific chemical structures of the GNRs, such as whether they contain other types of edge configurations. The square-root model only predicts the parity at  $k = \pi/b$ , but not that at  $k = 0$ . Regardless, the model guarantees a topological phase change by switching the direction of electric fields for a class of GNRs, given that the normal LUMO is occupied or the HOMO is unoccupied. Below we show another GNR to further demonstrate this point.

## 4 Another example of square-root GNR: 7-AGNR-S(1,3)

7-AGNR-S(1,3) shown in Fig. S6a is named according to the original publication [6]. The band structures in Fig. S6c, S6h, and S6j were obtained in the same way as in Fig. S5. The Zak phase for the middle four bands are labeled. We see the pattern agrees with case A and B in Table 1, which suggest a larger  $|t_1|$  than  $|t_2|$  (agrees with the original publication). For the corresponding square-root model, the parameters are chosen such that the gap width in Fig. S6f matches that in Fig. S6c, given that  $0 > t_2 > t_1$ , and  $m > 0$  for a positive electric field. Similar to pzc-GNR, with  $k = \pi/b$ , the two models give the same parity (see Fig. S6d and S6g, S6k and S6n). In addition, the parity at gamma point is also the same, which results in exactly the same Zak phase for the four bands in GNR and in square-root tight-binding model (see Fig. S6b and S6e, S6i and S6l). It shares the same topological feature as pzc-GNR that it has a phase change upon changing the direction of electric field with 203 or 205 occupied bands (The structure has 204 valence bands).

## 5 Boundary states in a finite molecule

In Fig. 4 of the main text we apply a step-function electric field described by

$$E = 0.2 \cdot \frac{2}{\pi} [\arctan(x/\epsilon) - \arctan((x - a_P/2)/\epsilon) + \arctan((x - a_P)/\epsilon)] (V/\text{\AA}) \quad (7)$$

where  $x$  is the horizontal coordinate and  $a_P$  is the length of the supercell equaling to 345.4 Å. The maximum field strength is thus 0.2 V/Å.  $\epsilon$  determines how abrupt the electric field changes sign and is denoted as the width of domain wall. The electrostatic potential added to electrons is then given by  $P = E \cdot (y - y_c)$ , where  $y_c$  is the vertical coordinate of the central atom. In this way we have equal number of electrons with positive and negative change of potential.

To simulate a finite molecule of pzc-GNR, we create a long molecule containing 10 unit cells with the two ends terminated by structures detected in experiments (Fig. S7e and S7f). We then apply a similar step-function according to  $0.2 \cdot \frac{2}{\pi} \arctan(x - a_F)$  (V/Å), where  $a_F$  is the length of the cell equaling to 250 Å. The GNR is placed such that the change of the field occurs at the boundary of the mirror symmetric unit cell (Fig. S7c). There are now two in-gap boundary states in total (Fig. S7a). The isosurfaces of the wave function of the two states are plotted in Fig. S7b and S7d.

## 6 Boundary states and choice of unit cell

There are two types of unit cell that can be drawn in pzc-GNR, one is mirror symmetric (Fig.1) and the other is not (Fig. S10b). The properties of boundary states depend on which unit cell the boundary is commensurate with. With mirror symmetric unit cell, boundary states are topologically protected and are degenerate. Fig. S8 illustrates the energy levels and spatial profile of boundary states calculated with DFT methods. Each of the finite gap owns a two-fold degenerate states with localized spatial distribution. The degeneracy remains regardless of the width of the domain wall (which is set to 0.5 Bohr and 4 Bohr in Fig. S8d and S8h, respectively). Fig. S8c is a replicate of Fig. 4a in the main text.

With the second choice of unit cell without mirror symmetry, localized boundary states can still be generated but they are no longer degenerate (Fig. S9a). Comparing Fig. S9a to Fig. S9e, it is obvious that the energy level is influenced by the width of domain wall. These properties can be expected by considering a Rice-Mele model described by

$$H(k) = \begin{pmatrix} m_r & 2t\cos(bk/2) \\ 2t\cos(bk/2) & -m_r \end{pmatrix} \quad (8)$$

where  $m_r$  is the on-site potential and  $t$  is the hopping parameter. Note the term Rice-Mele model can also refer to model with alternating hopping strength. In this work the name is used to refer to the Hamiltonian above.

With an non-mirror-symmetric unit cell, solitons from pzc-GNR behave similarly to solitons in a Rice-Mele model. Their structural similarity is shown Fig. S10. Soliton boundary states from Rice-Mele model have been well discussed before [8, 9]. Their existence is related to the nonsymmorphic chiral symmetry. The energy level is reported to be dependent on the width of domain wall. Here we use tight-binding model assuming nearest-neighbor hopping between carbon atoms only to simulate boundary states from GNRs when a step-function field is applied. Details of the tight-binding calculations have been mentioned in Sec. 3. The effect of the electric field is simulated by modifying the on-site potential of carbon atoms according to the coordinates of carbon atoms. The maximum strength of the electric field is adjusted so that

an effective gap (such as the one shown in Fig. S5c) of 0.2 eV is created for all GNRs. We also consider another GNR (5-sGNR [10]) that directly represents the Rice-Mele model when a transverse electric field is applied (Fig. S10a). It is named according to the original publication. The DFT calculated band structure of 5-sGNR is shown in Fig. S10e, which is consistent with previous report. The applied field with a strength of 0.3 V/Å can open up a gap of 0.09 eV at  $X$  near the Fermi level. The boundary states are thus expected to exist near the Fermi level.

In Fig. S11, it can be seen that boundary states in 5-sGNR and pzc-GNR with an non-mirror symmetric unit cell have similar behaviors. They indeed have a much stronger dependence on the width of domain wall, compared to pzc-GNR with mirror symmetric unit cell. A smoother domain wall pushes the energy of boundary states closer to the Fermi level (see inset in Fig. S11a and S11c). The width of domain wall also affects the spread of the boundary state, which can be evaluated by calculating the second moment of the wavefunction. Fig. S11b and S11f suggest a smoother domain yields a more localized boundary state for 5-sGNR, but a more spread state for pzc-GNR (with mirror symmetric terminating unit cell).

We further supplemented the above tight-binding results with DFT calculated boundary states in 5-sGNR. The electric field is applied as shown in Fig. S12 with the same width of domain wall as in Fig. S8 and S9. The maximum strength is 0.3 V/Å. The 0.5% isosurface of the wavefunction of the two boundary states are plotted in Fig. S12a and S12b, S12c and S12d with an abrupt and a smooth domain wall, respectively. A smoother domain wall results in an energy level slightly closer to the Fermi level, which is consistent with results obtained from the tight-binding method, although the energy dependency is not as obvious.

The above results imply that boundary states in 5-sGNR and non-mirror-symmetric pzc-GNR are of the same type, whereas they are different from mirror-symmetric square-root GNR. Although both types are localized and reside within gaps, they have a few distinctions. On one hand, the Rice-Mele type of boundary state can reside at the central gap, i.e., near the Fermi level, if there are only two zigzag segments in each unit cell, such as 5-sGNR. Samples don't have to be gated to observe boundary states. In comparison, the square-root type only exist at the finite gaps below or above the Fermi level. On the other hand, the square-root type of boundary states have robust quantized charge, resulting from quantized Zak phase due to mirror symmetry (Eq. S5), whereas Rice-Mele type does not. Depending on the specific requirements of potential applications, a square-root type, or a Rice-Mele type of boundary state can be chosen alternatively.

## References

- [1] Jacobse, P. H. *et al.* Tunable magnetic coupling in graphene nanoribbon quantum dots. *Small* 2400473 (2024).
- [2] Cayssol, J. & Fuchs, J.-N. Topological and geometrical aspects of band theory. *Journal of Physics: Materials* 4, 034007 (2021).

- 220 [3] McCann, E. Catalog of noninteracting tight-binding models with two energy  
221 bands in one dimension. *Physical Review B* **107**, 245401 (2023).
- 222 [4] Ryu, S., Schnyder, A. P., Furusaki, A. & Ludwig, A. W. Topological insulators  
223 and superconductors: tenfold way and dimensional hierarchy. *New Journal of*  
224 *Physics* **12**, 065010 (2010).
- 225 [5] Arkinstall, J., Teimourpour, M., Feng, L., El-Ganainy, R. & Schomerus, H. Topo-  
226 logical tight-binding models from nontrivial square roots. *Physical Review B* **95**,  
227 165109 (2017).
- 228 [6] Gröning, O. *et al.* Engineering of robust topological quantum phases in graphene  
229 nanoribbons. *Nature* **560**, 209–213 (2018).
- 230 [7] Yusufaly, T., Vanderbilt, D. & Coh, S. Tight-binding formalism in the context of  
231 the pythtb package (2013).
- 232 [8] Brzezicki, W. & Hyart, T. Topological domain wall states in a nonsymmorphic  
233 chiral chain. *Physical Review B* **101**, 235113 (2020).
- 234 [9] Allen, R. E., Gibbons, H. V., Sherlock, A. M., Stanfield, H. R. & McCann, E.  
235 Nonsymmorphic chiral symmetry and solitons in the rice-mele model. *Physical*  
236 *Review B* **106**, 165409 (2022).
- 237 [10] Rizzo, D. J. *et al.* Inducing metallicity in graphene nanoribbons via zero-mode  
238 superlattices. *Science* **369**, 1597–1603 (2020).
- 239 [11] Vo, T. H. *et al.* Large-scale solution synthesis of narrow graphene nanoribbons.  
240 *Nature communications* **5**, 3189 (2014).

Synthesis of compound 1: 5,10-dibromo-1,3-diphenyl-2H-cyclopenta[1]phenanthren-2-one (1) was synthesized according to a reported procedure [11].

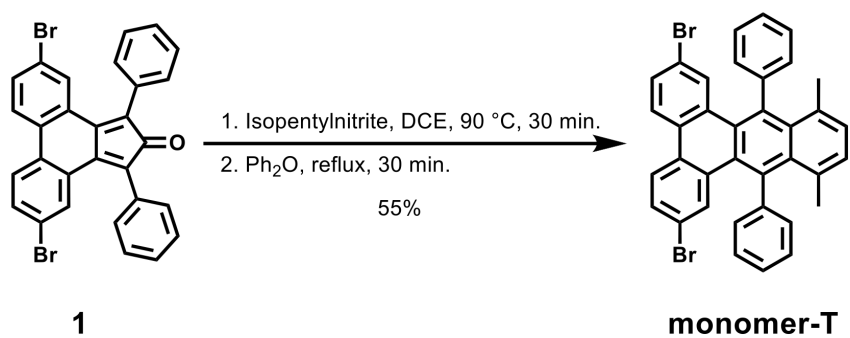

**Scheme S1.** Reaction scheme for the synthesis of monomer-T.

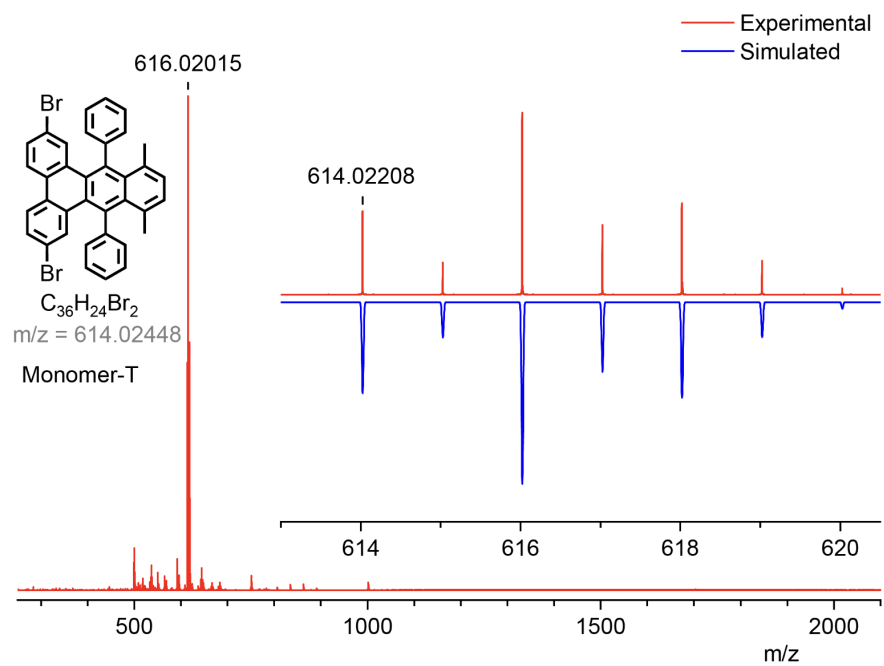

**Fig. S1** High-resolution (MALDI FT-ICR) mass spectrum of monomer-T (matrix: TCNQ). The insets show isotopic distributions for experimental and simulated spectra.

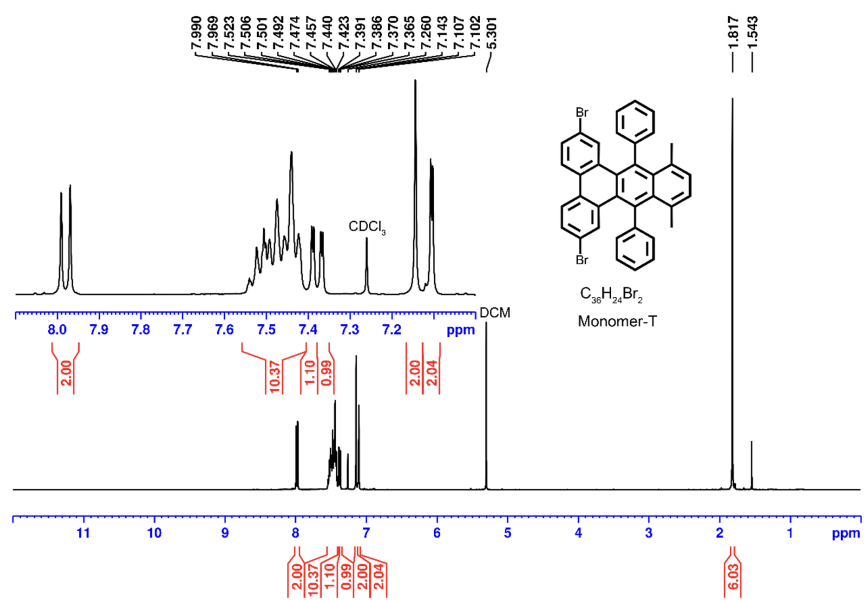

**Fig. S2**  $^1H$ -NMR (400MHz,  $CDCl_3$ ) of monomer-T.

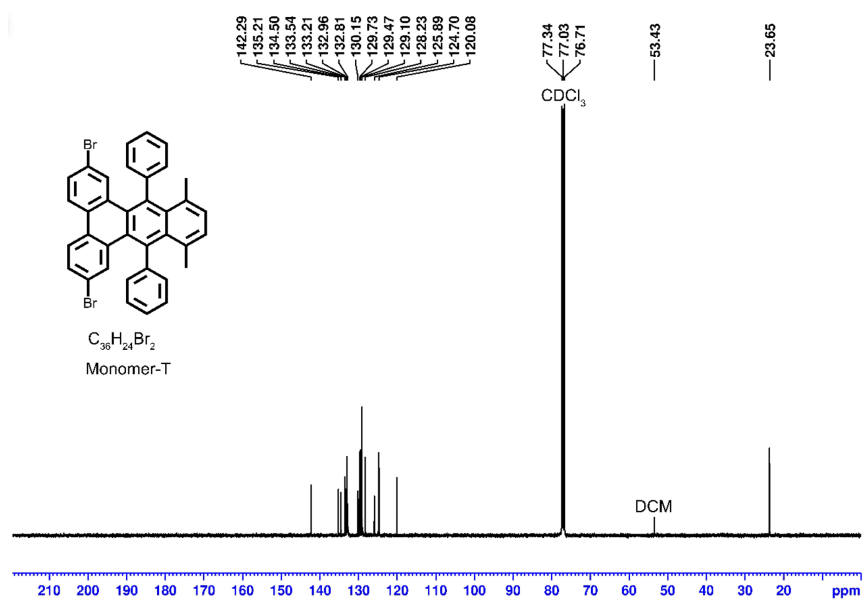

**Fig. S3**  $^{13}C$ -NMR (100MHz, CDCl<sub>3</sub>) of monomer-T.

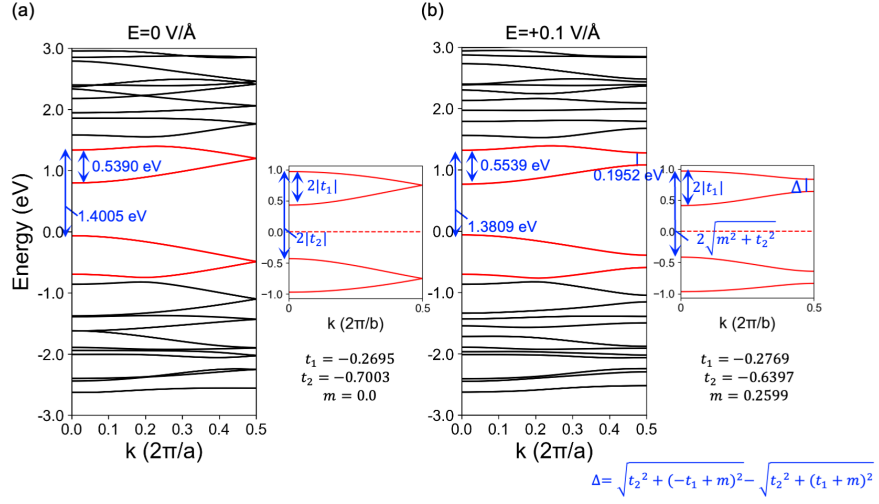

**Fig. S4** (a) Band structure of pzc-GNR without electric field calculated by DFT method, compared to the band structure of the tight-binding square-root model. The parameters for the square-root model are obtained by matching the gap width indicated in blue color. (b) Same comparison between band structures, with an electric field of 0.1 V/Å.

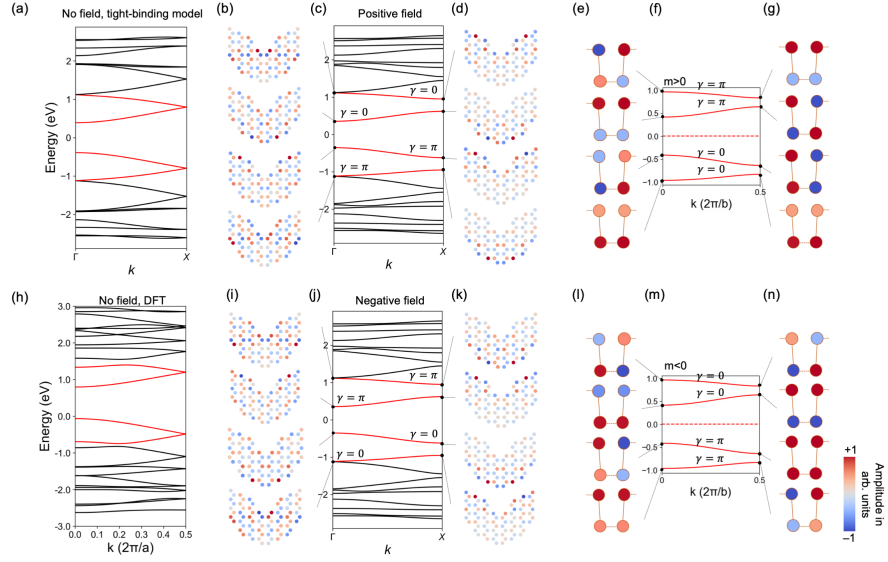

**Fig. S5** (a), (c), and (j) are band structures of pzc-GNR calculated in a tight-binding model assuming only nearest-neighbor hopping between carbon atoms. For comparison, (h) is the band structure calculated with DFT methods. (d) and (k) are plots of amplitude of the wave function for the four bands near the Fermi level at the middle of the Brillouin zone under a positive and negative electric field, respectively. Color stands for relative phase and saturation of color indicates strength of amplitude. (g) and (n) are amplitude of wave function calculated from the square-root model. They match well with (d) and (k). (b), (e), (i), (j) are the amplitude of wave function at the gamma point for the middle four bands. The square-root model only ensures the parity of wave function of GNR at  $X$ , but not at  $\Gamma$ .

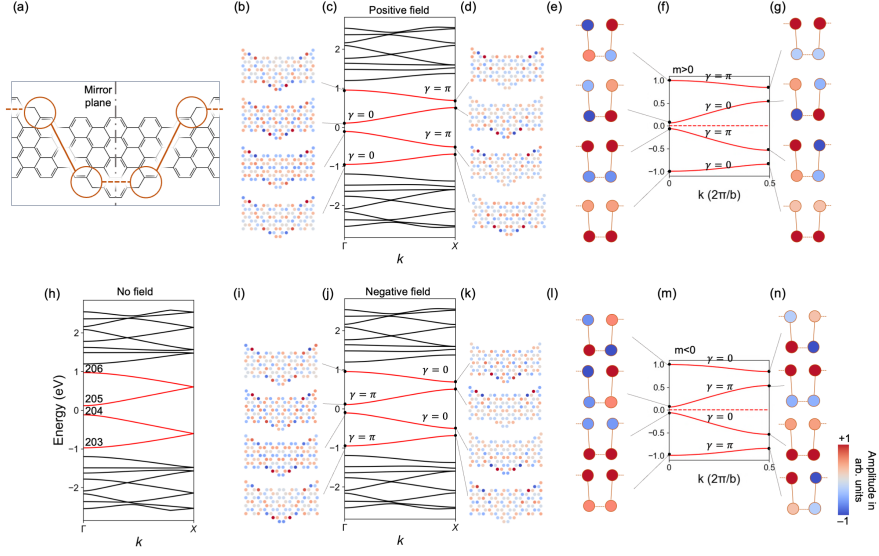

**Fig. S6** (a) Chemical structure of 7-AGNR-S(1,3). It has a mirror plane and four zigzag segments per unit cell. (c), (h), and (j) are band structures of 7-AGNR-S(1,3) calculated in a tight-binding model assuming only nearest-neighbor hopping between carbon atoms. (d) and (k) are plots of amplitude of the wave function for the four bands near the Fermi level at the middle of the Brillouin zone under a positive and negative electric field, respectively. Color stands for relative phase and saturation of color indicates strength of amplitude. (g) and (n) are amplitude of wave function calculated from the square-root model. They match well with (d) and (k). (b), (e), (i), (j) are the amplitude of wave function at the gamma point for the middle four bands. For this particular GNR, the parity of the middle four bands at both  $X$  and  $\Gamma$  match that in the square-root model. As a result, the Zak phases are exactly the same (e.g. see text in (c) and (f)).

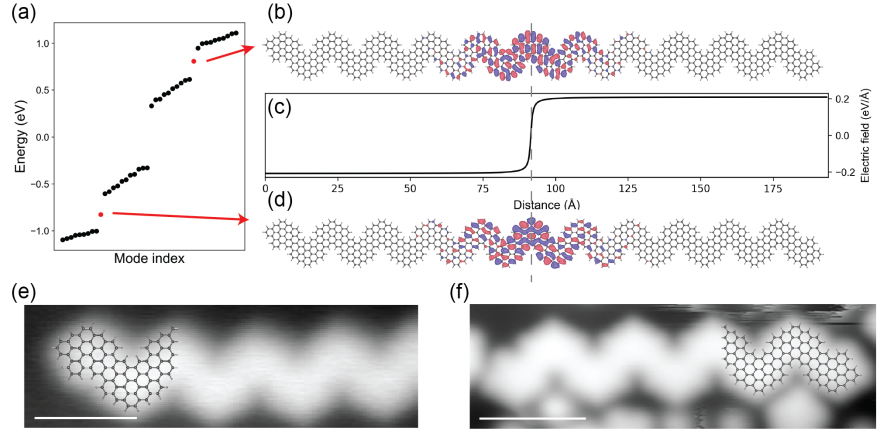

**Fig. S7** (a) Eigenvalues near the Fermi level for a finite molecule consisting of 10 repeating unit cells of pzc-GNR under a step-function electric field. The left and right terminating structures are drawn according to experimental observed STM images (see e and f). (c) Spatial profile of the externally applied electric field. (b) and (d) are 0.2% isosurfaces plots of the wave function residing at the upper finite gap, and the lower finite gap, respectively. They are localized at the interface where the switch of the electric field occurs. Scale bars: 2 nm.

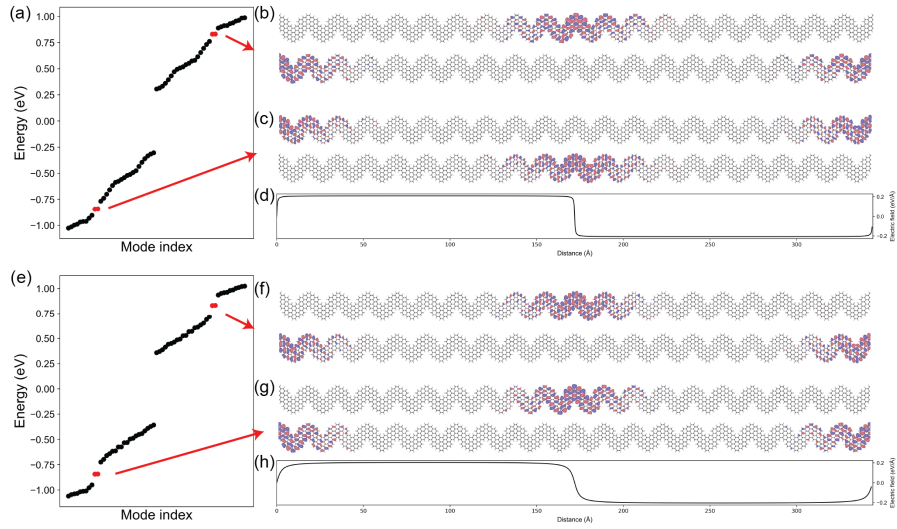

**Fig. S8** (a) Eigenvalues near the Fermi level for a supercell with 20 repeating unit cells of pzc-GNR under a step-function electric field with the spatial profile shown in (d). (b) and (c) are 0.5% isosurface plots of the wave function of boundary states residing at the upper finite gap, and the lower finite gap (red dots). They are localized at the interface where the switch of the electric field occurs (middle and the side of the supercell). Boundary states are two-fold degenerate in each finite gap. An electric field with a larger width of domain wall as illustrated in (h) is applied to the same supercell. Eigenvalues and corresponding localized boundary states are shown in (e), (f), and (g). Boundary states remain two-fold degenerate.

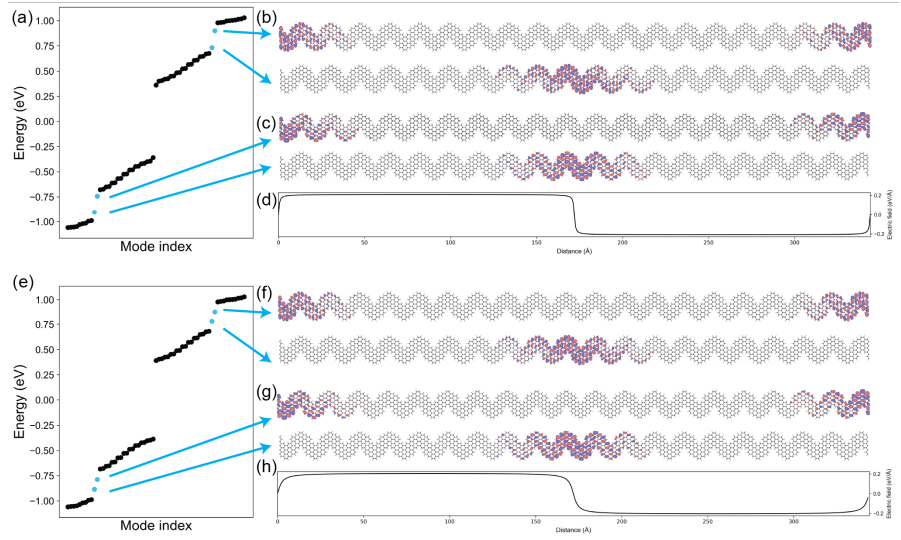

**Fig. S9** (a) Eigenvalues near the Fermi level for a supercell with 20 repeating unit cells of pzc-GNR under a step-function electric field with the spatial profile shown in (d). The unit cell is shifted from the one in Fig. S8 and is no longer mirror symmetric. (b) and (c) are 0.5% isosurface plots of the wave function of boundary states residing at the upper finite gap, and the lower finite gap (blue dots). They are localized at the interface and are nondegenerate. An electric field with a larger width of domain wall as illustrated in (h) is applied to the same supercell. Eigenvalues and corresponding localized boundary states are shown in (e), (f), and (g). Energy level of the boundary states is influenced by the width of the domain wall.

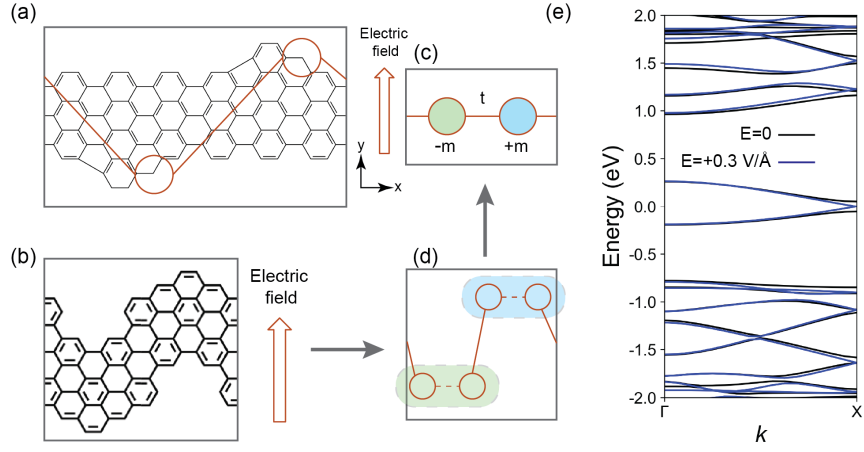

**Fig. S10** (a) Chemical structure of 5-sGNR as reported in [10]. (b) pzc-GNR drawn in a non-mirror symmetric unit cell. (c) Rice-Mele model with a nearest neighbor hopping of  $t$  and on-site potentials of  $-m$  and  $+m$ . (d) With the unit cell in (b), solitons from pzc-GNR behave in a similar way to that from the Rice-Mele model. (e) DFT calculated band structure of (a) with and without a transverse electric field. The applied field opens up a gap in the middle at  $X$ . The middle two bands can be explained by the Rice-Mele model (c). Energy is with respect to the Fermi level.

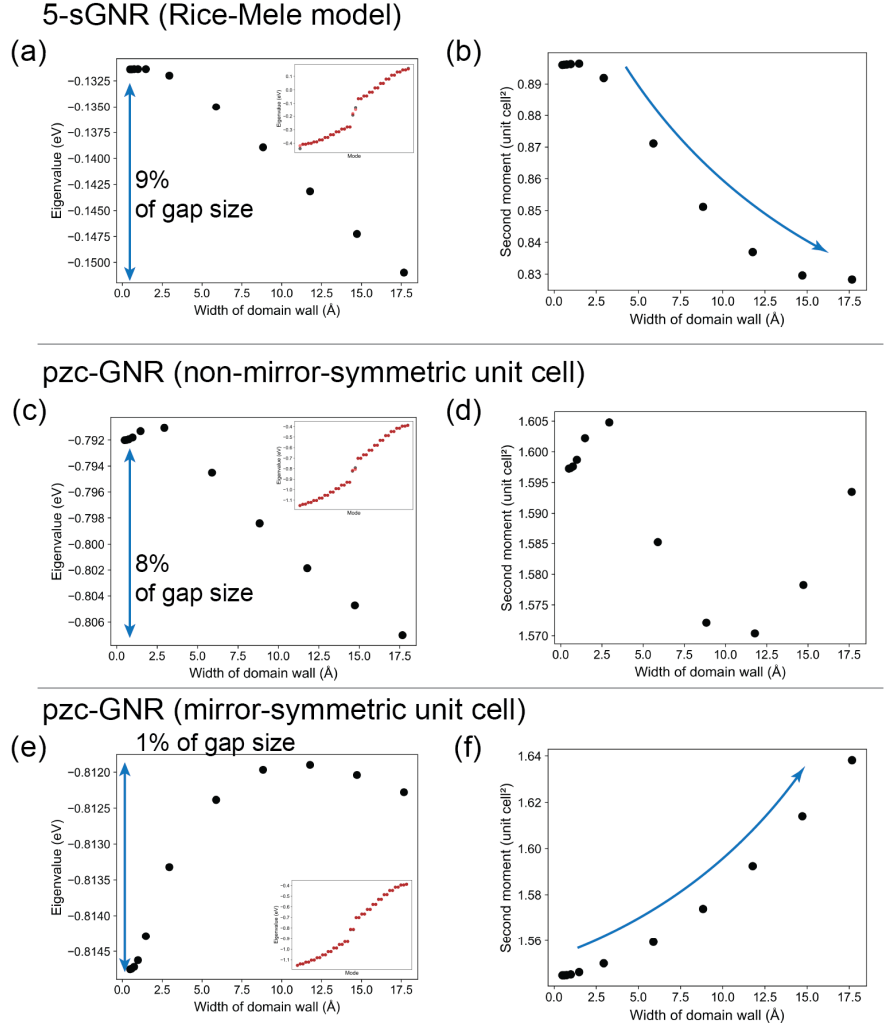

**Fig. S11** (a), (c), (e) are plots of energy levels of boundary states versus the width of domain wall for 5-sGNR, pzc-GNR with a mirror symmetric unit cell, and a non-mirror-symmetric unit cell, respectively. Insets show eigenvalues of modes near the center of the gap. Black and red correspond to the smallest and the largest width of domain wall considered. (b), (d), and (f) are corresponding plots of second moment of the boundary states versus the width of domain wall. Results are obtained by solving tight-binding Hamiltonian considering nearest-neighbour hopping between carbon atoms.

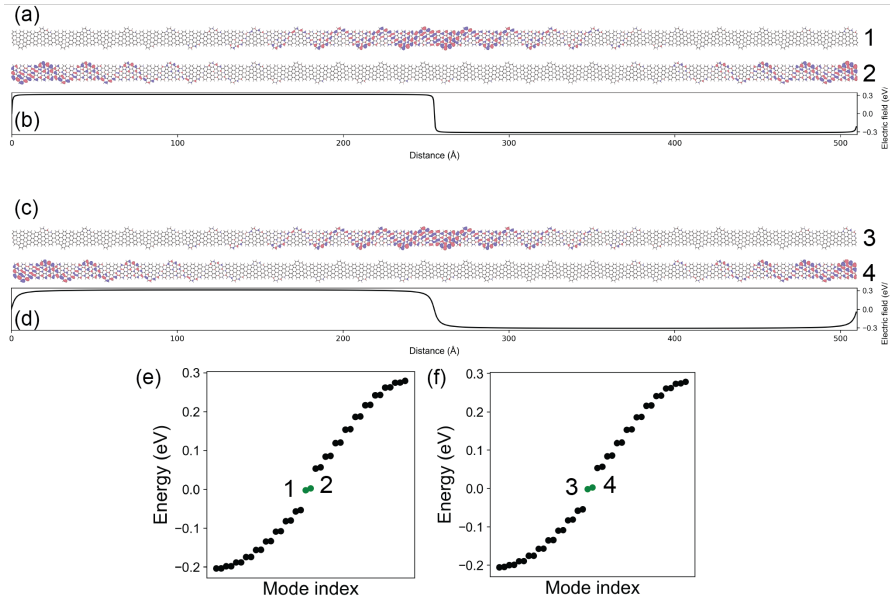

**Fig. S12** (a) 0.5% isosurfaces of wavefunctions of boundary states generated in 5-sGNR when a step-function electric field (b) is applied. The corresponding eigenvalues are shown in (e). (c) Same isosurface plot when a different electric field with a more smooth domain wall is applied (d). (f) Corresponding eigenvalues. Although not obvious, states number 3 and 4 are closer to zero comparing to 1 and 2.
